# Supplementary material for: Fully adaptive algorithm for pure exploration in linear bandits
Source: arXiv:1710.05552 source file (2017-10-16)
Supplement: Supplementary file 1 [file Appendix.tex]

\begin{lem}\label{lem:matrix-inequality}
Let $A$ be an positive definite matrix in  $\mathbb{R}^{d\times d}$ and $x,y$ be vectors in $\mathbb{R}^{d}$. Then, with any constant $\alpha > 0$, 
\[y^\top(A+\alpha xx^\top)^{-1}y \leq y^\top A^{-1}y\]
holds.
\end{lem}

\begin{proof}[Proof of Lemma \ref{lem:matrix-inequality}]
By Sherman{-}Morrison formula \citep{Sherman1950} we have, 
\begin{align*}
y^\top(A+\alpha xx^\top)^{-1}y &= y^\top\left(A^{-1} - \frac{\alpha A^{-1}xx^\top A^{-1}}{1+\alpha x^TA^{-1}x}\right)y\\
&= y^\top A^{-1}y - y^\top\frac{\alpha A^{-1}xx^\top A^{-1}}{1+\alpha x^TA^{-1}x}y\\
&\leq y^\top A^{-1}y.
\end{align*}
The last inequality follows from the fact that $A^{-1}$ is positive definite.
\end{proof}

\begin{lem}
\label{lem:complete-derivation}
Let $C_t$ be
\[C_t = R\sqrt{2\log\frac{K^2\det(A_t)^{\frac12}\det(\lambda I)^{-\frac12}}{\delta}} + \lambda^{\frac12}S.\]
Then,
\[\tau \leq H_\varepsilon C^2_\tau + K\]
means 
\begin{align}\label{eq:sample-complexity-2}
\tau \leq 8H_\varepsilon R^2\log\frac{K^2}{\delta} + C(H_\varepsilon,\delta),
\end{align}
where $C(H_\varepsilon,\delta)$ is
\[C(H_\varepsilon,\delta) = \mathcal{O}\left(H_\varepsilon\log\log\frac{1}{\delta}\right)\]
if $\lambda$ set smaller than
\begin{align}
\lambda \leq \frac{2R^2}{S^2}\log\frac{K^2}{\delta}. \label{eq:lambda-condition}
\end{align}
\end{lem}

\begin{proof}[Proof of Lemma \ref{lem:complete-derivation}]
By Proposition~\ref{prop:bound-of-confidence-interval}, we have 
\begin{align*}
C_\tau &\leq R\sqrt{2\log\frac{K^2}{\delta} + d\log\left(1+\frac{\tau L^2}{\lambda d}\right)}+\lambda^{\frac12}S \\
&\leq  2R\sqrt{2\log\frac{K^2}{\delta} + d\log\left(1+\frac{\tau L^2}{\lambda d}\right)}.
\end{align*}
The second inequality follows from condition \eqref{eq:lambda-condition}. Therefore, we can write
\begin{align*}
\tau &\leq H_\varepsilon C^2_\tau + K\\
&\leq 4H_\varepsilon R^2 \left(2\log\frac{K^2}{\delta} + d\log\left(1+\frac{\tau L^2}{\lambda d}\right)\right) + K.
\end{align*}

Let $\tau'$ be the parameter, which satisifies
\begin{align}
\tau = 4H_\varepsilon R^2 \left(2\log\frac{K^2}{\delta} + d\log\left(1+\frac{\tau' L^2}{\lambda d}\right)\right) + K.\label{eq:tau-bound}
\end{align}
Then, $\tau' \leq \tau$ holds. Let $N$ be defined as
\[N = 8H_\varepsilon R^2\log\frac{K^2}{\delta} + K,\]
and we have
\begin{align*}
\tau' &\leq \tau\\
&= 4H_\varepsilon R^2d\log\left(1+\frac{\tau'L^2}{\lambda d}\right)+ N\\
&\leq 4H_\varepsilon R^2\sqrt{dL^2\tau'/\lambda} + N.
\end{align*}
By solving this inequalty, we obtain
\begin{align*}
\sqrt{\tau'} &\leq  4H_\varepsilon R^2\sqrt{dL^2/\lambda} + \sqrt{16H^2_\varepsilon R^4dL^2\tau'/\lambda +N^2}\\
&\leq 2\sqrt{16H^2_\varepsilon R^4dL^2/\lambda +N^2}.
\end{align*}
Using this upper bound of $\tau'$ in \eqref{eq:tau-bound} yields
\[\tau \leq 8H_\varepsilon R^2\log\frac{K^2}{\delta} + \mathcal{O}\left(H_\varepsilon\log\log\frac{1}{\delta}\right).\]
\end{proof}

\begin{lem}
\label{lem:complete-derivation-2}
If $lambda$ is set as $\lambda > 2H_\varepsilon R^2L^2$, and $C_t$ is defined same as Lemma~\ref{lem:complete-derivation}, then
\[\tau \leq H_\varepsilon C^2_\tau + K\]
means 
\begin{align*}\tau \leq \left(1-\frac{2H_\varepsilon R^2L^2}{\lambda}\right)^{-1}\left(4H_\varepsilon R^2\log\frac{K^2}{\delta}  + C'\right),
\end{align*}
where $C'$ is
\[2H_\varepsilon\lambda S^2+K.\]
\end{lem}

\begin{proof}[Proof of Lemma~\ref{lem:complete-derivation-2}]
Again, by Proposition~\ref{prop:bound-of-confidence-interval}, we have
\begin{align*}
C_\tau &\leq R\sqrt{2\log\frac{K^2}{\delta} + d\log\left(1+\frac{\tau L^2}{\lambda d}\right)}+\lambda^{\frac12}S.
\end{align*}
From the fact $(a+b)^2 \leq a^2+b^2$ and $(1+\frac{1}{x})^x \leq e$, we have 
\begin{align*}
\tau &\leq H_\varepsilon C^2_\tau + K\\
&\leq 2H_\varepsilon \left(2R^2\log\frac{K^2}{\delta} + \frac{\tau R^2L^2}{\lambda} + \lambda S^2\right) + K.
\end{align*}
Therefore, we can conclude that if $\lambda > 2H_\varepsilon R^2L^2$, then
\begin{align*}
\tau \leq \left(1-\frac{2H_\varepsilon R^2L^2}{\lambda}\right)^{-1}\left(4H_\varepsilon R^2\log\frac{K^2}{\delta}  + C'\right),
\end{align*}
where $C'$ is
\[2H_\varepsilon\lambda S^2+K.\]

\end{proof}

\begin{proof}[Proof of Theorem \ref{thm:problem-complexity-bound}]
First, we bound the $\rho(y(i,j))$, which is the optimal value of
\begin{alignat}{2}
&\min_{p_k,w_k} & \sum_{k=1}& \frac{w_k^2}{p_k} \notag\\
&\mathrm{s.t.} &y(i,j)& = \sum_{k=1}^K w_kx_k\notag\\
&&\sum_{i=1}^K &\,p_k = 1,\, p_k\geq 0,\,p_k, w_k \in \mathbb{R}.\label{eq:4}
\end{alignat}
Now, since $y(i,j) = y(i,a^*) + y(a^*,j)$, the $p'_k$ and $w'_k$ defined as
\begin{align*}
&p'_k = \frac{p_k^*(y(i,a^*))+p^*_k(y(a^*,j))}{2}\\
&w'_k = w_k^*(y(i,a^*)) + w_k^*(y(a^*,j))
\end{align*}
satisfy the condition of \eqref{eq:4}. Therefore, we have
\begin{align*}
\rho(y(i,j)) &\leq \sum_{k=1} \frac{(w'_k)^2}{p'_k}\\
&= 2\sum_{k=1} \frac{( w_k^*(y(i,a^*)) + w_k^*(y(a^*,j)))^2}{p_k^*(y(i,a^*))+p^*_k(y(a^*,j))}\\
&\leq 4\sum_{k=1} \frac{( w_k^*(y(i,a^*)))^2 + (w_k^*(y(a^*,j)))^2}{p_k^*(y(i,a^*))+p^*_k(y(a^*,j))}\\
&\leq 4\sum_{k=1} \frac{( w_k^*(y(i,a^*)))^2 }{p_k^*(y(i,a^*))}+\frac{(  (w_k^*(y(a^*,j)))^2}{p^*_k(y(a^*,j))}\\
&= 4\rho(y(i,a^*))+4\rho(y(a^*,j)).
\end{align*}
Using this upper bound, we can bound the problem complexity $H_0$ as follows. Let $i^*(k)$ and $j^*(k)$ be defined as
\[(i^*_k,j^*_k) = \argmax_{i,j\in[K]}\frac{p^*_k(y(i,j))\rho(y(i,j))}{\max\left(\Delta_i^2,\Delta_j^2\right)}\]
and we have
\begin{align*}
H_0 &= 9\sum_{k=1}^K \max_{i,j\in[K]}\frac{p^*_k(y(i,j))\rho(y(i,j))}{\max\left(\Delta_i^2,\Delta_j^2\right)}\\
&= 9\sum_{k=1}^K \frac{p^*_k(y(i^*_k,j^*_k))\rho(y(i^*_k,j^*_k))}{\max\left(\Delta_{i^*_k}^2,\Delta_{j^*_k}^2\right)}\\
&\leq 36\sum_{k=1}^K p^*_k(y(i^*_k,j^*_k)) \frac{\rho(y(i^*_k,a^*))+\rho(a^*,j^*_k))}{\max\left(\Delta_{i^*_k}^2,\Delta_{j^*_k}^2\right)}\\
&\leq 36\sum_{k=1}^K p^*_k(y(i^*_k,j^*_k)) \left(\frac{\rho(y(i^*_k,a^*))}{\Delta_{i^*_k}^2}+\frac{\rho(a^*,j^*_k))}{\Delta_{j^*_k}^2}\right)\\
&\leq 72H'_{\text{oracle}}
\end{align*}
which was what we wanted. The last inequality holds from $\sum_{k=1}^K p^*_k(i,j) = 1$ for all $i,j\in[K]$
\end{proof}
